# Supplementary material for: Universal Backdoor Attacks Detection via Adaptive Adversarial Probe
Source: arXiv:2209.05244 source file (2022-12-07)
Supplement: Supplementary file 1 [file appendix.tex]

\section*{Appendix}
\appendix
\section{Experimental Setup}
\subsection{Clean Accuracy and Attack Success Rate for Experimental Models} We provide detailed information, including clean accuracy (C-ACC) and Attack Success Rate (ASR-b) \mr{duplicated with adversarial attack} for each attack method on all three datasets (shown in Table \ref{table:models information}). It is worth noting that in order to ensure a high ASR-b for each attack method, we make several adjustments in model training. Specifically, we avoid adopting MobileNet-V2 when using WaNet since we find a weak ASR-b during training. We also set the trigger transparency to 1 when testing both the Blend-h and Blend-l attack. 

\subsection{Backdoor Attack} We explain how we inject backdoor to models with various trigger patterns in the paper. For all BadNets models, we utilize white squares as the backdoor trigger and randomly select a position (Top-Left, Top-Right, Bottom-Right and Bottom-Left) to patch the trigger pattern. For both CIFAR-10 and GTSRB, we utilize $4 \times 4$ trigger to poison training dataset in BadNets-s setting and utilize $6 \times 6$ trigger in BadNets-l setting. For Tiny-ImageNet, we also use $4 \times 4$ trigger in BadNets-s. However, we change the trigger size to $10 \times 10$ since images from Tiny-ImageNet take a larger resolution to $64 \times 64$ compared with the resolution of $32 \times 32$ in CIFAR-10 and GTSRB.

\begin{table}
\centering
\caption{Comparison of budget increment measure.}
\begin{tabular}{llll} 
\hline
\textbf{Measure} & \textbf{ACC(\%)} & \textbf{Avg Time(s)}\\ 
\hline
Cumulatively         & \textbf{85.000}       & 82.453        \\
Exponentially           & 82.500   & \textbf{20.333}  \\
\hline
\end{tabular}
\label{table:comparison of budget increment measure}
\end{table}

\begin{table}
\centering
\caption{Attack Information.}
\begin{tabular}{llll} 
\hline
\textbf{Dataset}               & \textbf{Attack} & \textbf{ASR-b(\%)} & \textbf{C-ACC(\%)}            \\ 
\hline
\multirow{6}{*}{CIFAR-10}      & BadNets-s                & 94.95        & \multirow{6}{*}{85.41}  \\
                               & BadNets-l                & 95.01        &                         \\
                               & Blend-h                  & 99.14        &                         \\
                               & Blend-l                  & 99.84        &                         \\
                               & WaNet                    & 90.35        &                         \\
                               & Input-aware              & 86.47        &                         \\ 
\hline
\multirow{6}{*}{GTSRB}         & BadNets-s                & 93.38        & \multirow{6}{*}{93.54}  \\
                               & BadNets-l                & 93.77        &                         \\
                               & Blend-h                  & 99.27        &                         \\
                               & Blend-l                  & 99.82        &                         \\
                               & WaNet                    & 88.48        &                         \\
                               & Input-aware              & 86.49        &                         \\ 
\hline
\multirow{6}{*}{Tiny-ImageNet} & BadNets-s                & 100.0        & \multirow{6}{*}{50.10}  \\
                               & BadNets-l                & 100.0        &                         \\
                               & Blend-h                  & 99.23        &                         \\
                               & Blend-l                  & 99.64        &                         \\
                               & WaNet                    & 99.40        &                         \\
                               & Input-aware              & 99.42        &                        
\end{tabular}
\label{table:models information}
\end{table}

\subsection{Evaluation Metrics} We utilize three evaluation metrics in the paper: the detection accuracy (ACC), the AUROC and Average Attacks. ACC illustrates our method's ability in backdoor models with a specific dataset and model architecture. A high ACC represents the robustness to backdoor attacks. AUROC measures the comprehensive performance of both backdoor and benign models. A high AUROC illustrates that the detection method is unlikely to predict a clean model as backdoor model under the same ACC. Apart from the two commonly used metrics, we also introduce the Average Attacks which shows the general detection ability across different attack methods. A high Average Attacks means the detection is much more robust against backdoor attacks, thus is more practical in real detection scenarios.\section{Discussion on Budget Increment Measure}
 In the proposed A2P, we generate the optimal perturbation via adaptively adjusting the region and budget of the adversarial attack. To search for a suitable budget, we design two kinds of measures in either cumulative (+ 2) or exponential ($\times$ 2) way and make a comparison between them. 

We first investigate the visual similarity between perturbations generated by two incremental measures and trigger patterns. Figure \ref{fig:budget_increment_measure} shows the relationship between budget and trigger patterns. From top to bottom, two perturbations are generated by the big $\epsilon$-ball constraint and the small $\epsilon$-ball constraint, respectively. We observe that perturbations under different $\epsilon$-ball are similar to different trigger patterns visually, especially for perturbation-based backdoor attacks. Figure \ref{fig:incremental_comp} shows the comparison of cumulatively increment and exponentially increment, demonstrating that the perturbation generated by cumulatively increment is more similar to the last iteration than the perturbation generated by exponentially increment and takes more stages to grow to 1 for cumulatively increment, which reduces the detection efficiency. 

We further conduct experiments to compare two incremental measures. We utilize 40 BadNet models on CIFAR-10 with ResNet-18 to compare the ACC and average computational overhead for a model between two measures and set the ratio of the region to 0.005. Notably, we stop the detection process when threshold $\tau \ge 3.5$. As shown in Table \ref{table:comparison of budget increment measure}, both measures contribute to good detection performance with ACC $\ge$ 82.5\%, while exponential measure is much faster than cumulative measure. We also notice that exponential measure costs less time than the cumulative measure. As a result, we use the exponential budget increment measure in the paper. 

\section{Alleviating Backdoor through Model Unlearning}
\section{Detection of Multiple Triggers within Single Image}
In this section, we test the detection performance of our A2P on rigorous scenarios consisting of different trigger sizes and transparencies. We further verify A2P on another rigorous scenario: multiple triggers in one sample. Figure \ref{fig:multiple triggers} shows some samples with multiple trigger(from 1 to 5). We train 10 BadNet models on CIFAR-10 with ResNet-18 for each trigger number setting. Notably, we utilize triggers with more complex colors. Figure \ref{fig:multiple triggers result} shows the result of multiple triggers in one sample. We demonstrate that the ACC will drop as the trigger number increases. However, when the trigger number is up to 5, ACC performs better again. Especially, NC is more stable in the multiple triggers scenario, while DF-TND has poor performance with ACC $\le 10\%$. We further observe that A2P will identify another specific label as the latent backdoor in early stages. We deem that excessive adversarial attack will disturb the detection performance, while A2P and DF-TND are based on adversarial attacks. We leave this problem to our future work.
% \section{Experiments on Different Threat Model}
% In this section, we mainly focus on the possible effect brought by the different threat models of adversarial attack. For simplicity, we compare two types of adversarial perturbations bounded by $\ell_{\infty}$-ball and $\ell_{2}$-ball and our results are shown in ...
\section{hyper-parameter}

\section{ Budget Mapping Measure }

\section{ Model drawback }

\section{ formulate to optimization problem, using gradient descent. core: loss / adv turn to one step}

\textbf{Adversarial Perturbation Magnitude.} The magnitude of generated adversarial perturbations play an important role in the overall detection framework. To better study this, we compare two types of adversarial perturbations bounded by $\ell_{\infty}$-norm and $\ell_{2}$-norm. Specifically, we use 30 infected models by BadNet and 30 clean models, both of which are trained on CIFAR-10 with ResNet-18. As shown in \ref{fig:rest ablation study} (b), we could observe that both $\ell_{\infty}$-ball and $\ell_{2}$-ball constraints can achieve high performance with ROC $\ge 0.97$. (??? the conclusion is meaningless)
